# Supplementary material for: Quantum corrections in nanoplasmonics: shape, scale, and material
Source: arXiv:1608.05421 ancillary file (2016-08-30)
Supplement: Supplementary file 1 [file SupportingMaterial.pdf]

# SUPPORTING MATERIAL

## Quantum corrections in nanoplasmonics: shape, scale, and material

Thomas Christensen,[1] Wei Yan,[2] Antti-Pekka Jauho,[3,4] Marin Soljačić,[1] and N. Asger Mortensen[4,5]
[1] *Department of Physics, Massachusetts Institute of Technology, Cambridge, Massachusetts, USA*
[2] *Institut d'Optique d'Aquitaine, Université Bordeaux, CNRS, 33405 Talence, France*
[3] *Department of Micro- and Nanotechnology, Technical University of Denmark, 2800 Kgs. Lyngby, Denmark*
[4] *Center for Nanostructured Graphene, Technical University of Denmark, 2800 Kgs. Lyngby, Denmark*
[5] *Department of Photonics Engineering, Technical University of Denmark, 2800 Kgs. Lyngby, Denmark*

### I. REFLECTION FROM A PLANAR INTERFACE: THE FEIBELMAN $d$-PARAMETERS

The use of the Feibelman $d_\perp$- and $d_\parallel$-parameters for the planar single-interface system is well-established and indeed presented in numerous excellent accounts [S1–S4]. Even so, we here offer a short and concise introduction for the interested reader, whose outlook, to the best of our knowledge, is complementary to existing accounts. Our motivation in doing so is twofold: firstly, to provide a maximally self-contained and accessible treatment, and secondly, to cast the foundations in explicit terms without implicit conventions or hidden assumptions.

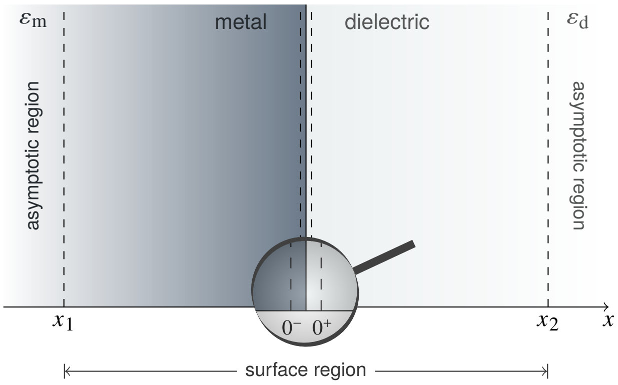


FIG. S1 Schematic illustration of the distinct regions in the analysis leading to the Feibelman $d$-parameters.

The approach chosen here to introduce the $d$-parameters is conceptually straightforward: derive the lowest-order nonclassical corrections to the classical reflection coefficient for the nonretarded potentials, $r^c = -\frac{\varepsilon_m - \varepsilon_d}{\varepsilon_m + \varepsilon_d}$, for reflection off a planar interface at $x = 0$ separating metallic ($x < 0$) and dielectric ($x > 0$) regions with associated local bulk permittivities $\varepsilon_m$ and $\varepsilon_d$, respectively, as indicated in Fig. S1. To do so, we consider perturbation of the system by an external potential $\phi^{ext}(\mathbf{r}) = e^{iky+kx}$, corresponding to excitation by a field of momentum $k$ impinging from the dielectric region. In response to this perturbation a (surface-peaked) charge density deviation $\rho(\mathbf{r}) = \rho(x)e^{iky}$ is instated,[1] whose evaluation in general requires a full quantum-mechanical treatment. The associated induced potential $\phi^{ind}(\mathbf{r}) = \phi^{ind}(x)e^{iky}$

[1] We emphasize that this charge density includes *both* bound and free charges; this point is further discussed in Section VI.

follows directly from $\rho(x)$ via Coulomb's law[2]

$$\phi^{\mathrm{ind}}(x) = \frac{1}{2\varepsilon_0 k} \int_{x_1}^{x_2} \mathrm{e}^{-k|x-x'|} \rho(x')\,\mathrm{d}x', \tag{S1}$$

where $x_1$ and $x_2$ indicate positions far from the interface where the charge density has effectively vanished, see Fig. S1. The asymptotic behavior of the induced potential beyond $x_1$ and $x_2$ can be well-described for surface-peaked charge densities by expanding around $qx' = 0$, thereby effectively introducing a multipole expansion:

$$\begin{aligned}\phi^{\mathrm{ind}}(x) &= \frac{\mathrm{e}^{-k|x|}}{2\varepsilon_0 k} \int_{x_1}^{x_2} \Big\{1 + \mathrm{sgn}(x)kx' + O\big[(kx')^2\big]\Big\}\rho(x')\,\mathrm{d}x' \\ &= \frac{\mathrm{e}^{-k|x|}}{2\varepsilon_0 k}\sigma\Big\{1 + \mathrm{sgn}(x)kd_\perp + O\big[(kX)^2\big]\Big\},\end{aligned} \tag{S2}$$

with a (by ansatz small) generic length scale $X$, and with monopole and dipole moments $\sigma$ and $d_\perp$:

$$\sigma \equiv \int_{x_1}^{x_2} \rho(x)\,\mathrm{d}x, \qquad d_\perp \equiv \frac{1}{\sigma}\int_{x_1}^{x_2} x\rho(x)\,\mathrm{d}x, \tag{S3}$$

corresponding, respectively, to the effective (quantum mechanical) surface charge density and to the position of the centroid of induced charge.

Aiming to obtain far-field reflection properties with nonclassical corrections of order $O(kX)$ we define an asymptotic (or, auxiliary) potential $\phi^\infty(x)$ which agrees with the actual total potential $\phi^{\mathrm{ext}}(x) + \phi^{\mathrm{ind}}(x)$ in the far-field asymptotic regions where $|x| \geq |x_{1,2}|$

$$\phi^\infty(x > 0) \equiv \mathrm{e}^{kx} + r\mathrm{e}^{-kx}, \qquad \phi^\infty(x < 0) \equiv t\mathrm{e}^{kx}, \tag{S4a}$$

expressed in terms of coefficients $r$ and $t$ that follow directly from Eq. (S2):

$$r = \frac{1}{2\varepsilon_0 k}\sigma(1 + kd_\perp), \qquad t = 1 + \frac{1}{2\varepsilon_0 k}\sigma(1 - kd_\perp). \tag{S4b}$$

Although this auxiliary potential corresponds to a physical reality only in the asymptotic regions, we can conceptually extend their range of validity into the surface region $|x| < |x_{1,2}|$, thereby allowing us to interpret $r$ and $t$ as semiclassical reflection and transmission coefficients, respectively. An appreciation of their relation to their classical counterparts requires a disentangling of the implicit material-dependence hidden in $\sigma$. To achieve this disentangling requires two steps, amounting essentially to the derivation of a set of modified boundary conditions (BCs).

1. *Continuity of $\phi^\infty$ across $x = 0$.* By subtracting potential components on either side of the interface, i.e. $\phi^\infty(x = 0^-) + \phi^\infty(x = 0^+)$, while utilizing Eq. (S4a), we obtain a generalization of the usual classical BC of continuity of the potential, which is instead supplanted by:

$$\phi^\infty(0^+) - \phi^\infty(0^-) = 1 + r - t = \frac{\sigma d_\perp}{\varepsilon_0}. \tag{S5}$$

*Derivative of $\phi^\infty$ across $x = 0$.* The auxiliary potentials obey a generalized Poisson equation,

$$\varepsilon_0 \nabla^2 \phi^\infty(\mathbf{r}) = -\tilde{\rho}(\mathbf{r}) + \boldsymbol{\nabla}\cdot\mathbf{P}(\mathbf{r}), \tag{S6}$$

---

[2] This particular form follows upon integrating out the $y'$- and $z'$-dependencies in $\phi^{\mathrm{ind}}(\mathbf{r}) = \frac{1}{4\pi\varepsilon_0}\iiint_{-\infty}^{\infty} \frac{1}{|\mathbf{r}-\mathbf{r}'|}\rho(x')\mathrm{e}^{\mathrm{i}ky'}\,\mathrm{d}x'\,\mathrm{d}y'\,\mathrm{d}z'$, yielding $\phi^{\mathrm{ind}}(\mathbf{r}) = \frac{1}{\pi\varepsilon_0}\mathrm{e}^{\mathrm{i}ky}\int_{-\infty}^{\infty}\Big\{\int_0^\infty K_0\big[k\sqrt{(x-x')^2+\tilde{z}^2}\big]\,\mathrm{d}\tilde{z}\Big\}\rho(x')\,\mathrm{d}x' = \frac{1}{2\varepsilon_0 k}\mathrm{e}^{\mathrm{i}ky}\int_{-\infty}^{\infty}\mathrm{e}^{-k|x-x'|}\rho(x')\,\mathrm{d}x'$ (using the integral identities $\int_{-\infty}^{\infty}(\tilde{x}^2+\tilde{y}^2+\tilde{z}^2)^{-1/2}\mathrm{e}^{\mathrm{i}k\tilde{y}}\,\mathrm{d}\tilde{y} = 2K_0\big(k\sqrt{\tilde{x}^2+\tilde{z}^2}\big)$ and $\int_0^\infty K_0\big(k\sqrt{\tilde{x}^2+\tilde{z}^2}\big)\,\mathrm{d}\tilde{z} = \frac{\pi}{2k}\mathrm{e}^{-k|\tilde{x}|}$ [S5, Eqs. 3.754.2 & 6.596.3]).

with effective charge and dipole densities $\tilde{\rho}(\mathbf{r}) \equiv \sigma\delta(x)\mathrm{e}^{\mathrm{i}ky}$ and $\mathbf{P}(\mathbf{r}) \equiv \sigma d_\perp\delta(x)\mathrm{e}^{\mathrm{i}ky}\hat{\mathbf{x}}$,[3] representing the contributions from zeroth and first moments of the actual induced charge $\rho(\mathbf{r})$. By integrating Eq. (S6) over the infinitesimal interval $x \in [0^-, 0^+]$ we obtain an additional BC:

$$\begin{aligned}\partial_x\phi^\infty(x=0^+) - \partial_x\phi^\infty(x=0^-) &= -\frac{\sigma}{\varepsilon_0} \\ \Leftrightarrow 1 - r - t &= -\frac{\sigma}{\varepsilon_0 k},\end{aligned} \tag{S7}$$

which is just the conventional classical result.

*First effective boundary condition.* By combining Eqs. (S5) and (S7) we obtain the first of two equations which interrelate $r$ and $t$ without reference to $\sigma$:

$$(1 + kd_\perp) + r(1 - kd_\perp) - t(1 + kd_\perp) = 0. \tag{S8}$$

2. *Auxiliary classical charge and current densitities.* The second step involves the introduction of classical constitutive parameters, namely the bulk dielectric functions $\varepsilon_{\mathrm{m,d}}$. To that end, we consider a set of auxiliary *classical* charge and current densities, $\rho^\infty(\mathbf{r})$ and $\mathbf{J}^\infty(\mathbf{r})$, mutually interrelated by a continuity equation $\boldsymbol{\nabla}\cdot\mathbf{J}^\infty(\mathbf{r}) - \mathrm{i}\omega\rho^\infty(\mathbf{r}) = 0$, and jointly subject to the asymptotic condition that $\mathbf{J}^\infty(\mathbf{r})$ approaches the actual quantum mechanical current $\mathbf{J}(\mathbf{r})$ in the asymptotic regions $|x| \geq |x_{1,2}|$. With the current components $\mathbf{J}^\infty(\mathbf{r}) \equiv [\mathrm{J}_x^\infty(x), \mathrm{J}_y^\infty(x), 0]^\mathrm{T}\mathrm{e}^{\mathrm{i}ky}$ and a surface-charge ansatz for the charge density $\rho^\infty(\mathbf{r}) \equiv \sigma^\infty\delta(x)\mathrm{e}^{\mathrm{i}ky}$ the continuity equation can be integrated from $x = 0^-$ to $x = 0^+$, producing:

$$\mathrm{i}\omega\sigma^\infty = \int_{0^-}^{0^+} \partial_x\mathrm{J}_x^\infty(x) + \mathrm{i}k\mathrm{J}_y^\infty(x)\,\mathrm{d}x = \mathrm{J}_x^\infty(0^+) - \mathrm{J}_x^\infty(0^-) + \mathrm{i}k\int_{0^-}^{0^+}\mathrm{J}_y^\infty(x)\,\mathrm{d}x = \mathrm{J}_x^\infty(0^+) - \mathrm{J}_x^\infty(0^-),$$

where the integral over $\mathrm{J}_y^\infty(x)$ vanishes since the integrand is nonsingular and the domain infinitesimal. By definition, $\mathrm{J}_x^\infty(0^\pm)$ represent classical current densities; consequently, they are generated by the asymptotic fields through classical bulk conductivities $-\mathrm{i}\omega\varepsilon_0[\varepsilon(x) - 1]$ (including free *and* bound carriers) with $\varepsilon(x < 0) = \varepsilon_\mathrm{m}$ and $\varepsilon(x > 0) = \varepsilon_\mathrm{d}$, such that:

$$\begin{aligned}\sigma^\infty &= \varepsilon_0(\varepsilon_\mathrm{d} - 1)\partial_x\phi^\infty(x=0^+) - \varepsilon_0(\varepsilon_\mathrm{m} - 1)\partial_x\phi^\infty(x=0^-) \\ \Leftrightarrow (\varepsilon_\mathrm{d} - 1)(1 - r) - (\varepsilon_\mathrm{m} - 1)t &= \frac{\sigma^\infty}{\varepsilon_0 k}.\end{aligned} \tag{S9}$$

*Introducing the $d_\parallel$-parameter.* The usefulness of Eq. (S9) hinges upon a well-defined relationship between the asymptotic and actual surface charge densities $\sigma^\infty$ and $\sigma$, respectively. Such a relationship can be obtained by exploiting the asymptotic equality between $\mathbf{J}^\infty$ and $\mathbf{J}$. Concretely, by integrating the continuity equation of the (asymptotic) actual charge and current densities, $\{\rho^{(\infty)}, \mathbf{J}^{(\infty)}\}$, over a domain extending into the asymptotic region, i.e. over $x \in [x_1, x_2]$, one obtains:

$$\mathrm{i}\omega\sigma^{(\infty)} = \mathrm{J}_x^{(\infty)}(x_2) - \mathrm{J}_x^{(\infty)}(x_1) + \mathrm{i}k\int_{x_1}^{x_2}\mathrm{J}_y^{(\infty)}(x)\,\mathrm{d}x. \tag{S10}$$

Then, using this relation, we subtract $\sigma^\infty$ from $\sigma$ and thereby obtain the desired relationship:

$$\begin{aligned}\mathrm{i}\omega(\sigma - \sigma^\infty) &= \big[\mathrm{J}_x(x_2) - \mathrm{J}_x^\infty(x_2)\big] - \big[\mathrm{J}_x(x_1) - \mathrm{J}_x^\infty(x_1)\big] + \mathrm{i}k\int_{x_1}^{x_2}\big[\mathrm{J}_y(x) - \mathrm{J}_y^\infty(x)\big]\,\mathrm{d}x \\ \Leftrightarrow \sigma &= \sigma^\infty + \frac{k}{\omega}\int_{x_1}^{x_2}\big[\mathrm{J}_y(x) - \mathrm{J}_y^\infty(x)\big]\,\mathrm{d}x,\end{aligned} \tag{S11}$$

[3] This can be established by inserting $\phi^\infty(\mathbf{r})$ from Eq. (S2) into (S6), while utilizing that $\nabla^2\mathrm{e}^{-k|x|+\mathrm{i}ky} = -2k\delta(x)\mathrm{e}^{\mathrm{i}ky}$ and $\nabla^2\big[\mathrm{sgn}(x)\mathrm{e}^{-k|x|+\mathrm{i}ky}\big] = 2\delta'(x)\mathrm{e}^{\mathrm{i}ky}$ [derivable e.g. from a weak limit form of the Dirac delta function and its (anti-)derivatives].

where the terms $J_x(x_{1,2}) - J_x^\infty(x_{1,2})$ vanish by virtue of the asymptotic condition $\mathbf{J}^\infty(x) = \mathbf{J}(x)$ which applies for $|x| \geq |x_{1,2}|$. At this point, we introduce Feibelman's parallel $d$-parameter:

$$d_\parallel \equiv \frac{\int_{x_1}^{x_2} \left[J_y(x) - J_y^\infty(x)\right] \mathrm{d}x}{J_y^\infty(0^-) - J_y^\infty(0^+)}. \tag{S12}$$

Crucially, the $d_\parallel$-parameter can be rewritten as a function of only the quantum mechanical current density, see Section I.B, i.e. without explicit referencing of the asymptotic fields. Moreover, by a slight rearrangement of its definition, a useful rephrasing of the integral term in Eq. (S11) is achieved:

$$\int_{x_1}^{x_2} \left[J_y(x) - J_y^\infty(x)\right] \mathrm{d}x = d_\parallel\left[J_y^\infty(0^-) - J_y^\infty(0^+)\right] = kd_\parallel\omega\varepsilon_0\left[(1-\varepsilon_\mathrm{m})t + (\varepsilon_\mathrm{d} - 1)(1+r)\right],$$

which allows re-expressing Eq. (S11) as:

$$\sigma = \sigma^\infty + k^2 d_\parallel \varepsilon_0\left[(1-\varepsilon_\mathrm{m})t + (\varepsilon_\mathrm{d} - 1)(1+r)\right]. \tag{S13}$$

*Second effective boundary condition.* Finally, to obtain the second and final equation which interrelates $r$ and $t$, and thus complements Eq. (S8), we substitute into (S13), replacing $\sigma^\infty$ via (S9) and $\sigma$ via (S7), which, after some manipulation, leads to:

$$[\varepsilon_\mathrm{d}(1 + kd_\parallel) - kd_\parallel] - [\varepsilon_\mathrm{d}(1 - kd_\parallel) + kd_\parallel]r - [\varepsilon_\mathrm{m}(1 + kd_\parallel) - kd_\parallel]t = 0. \tag{S14}$$

Equations (S8) and (S14) constitute two coupled equations for the asymptotic reflection and transmission coefficients $r$ and $t$; by solving them we can obtain the first-order quantum mechanical generalization of the classical coefficients $r^\mathrm{c}$ and $t^\mathrm{c}$:

$$r = -\frac{(\varepsilon_\mathrm{m} - \varepsilon_\mathrm{d}) + (\varepsilon_\mathrm{m} - \varepsilon_\mathrm{d})k(d_\perp + d_\parallel)}{(\varepsilon_\mathrm{m} + \varepsilon_\mathrm{d}) - (\varepsilon_\mathrm{m} - \varepsilon_\mathrm{d})k(d_\perp - d_\parallel)}, \tag{S15a}$$

$$t = \frac{2\varepsilon_\mathrm{d}}{(\varepsilon_\mathrm{m} + \varepsilon_\mathrm{d}) - (\varepsilon_\mathrm{m} - \varepsilon_\mathrm{d})k(d_\perp - d_\parallel)}, \tag{S15b}$$

retaining terms only up to linear order in $kd_{\perp,\parallel}$ in the fraction.

### A. Equivalent boundary conditions at arbitrary surfaces

Aspects of the preceding discussion hint that the Feibelman $d$-parameters may be interpreted in terms of auxiliary, effective boundary terms. This is particularly clear in the case of the $d_\perp$-parameter; its emergence at first order in a multipole analysis suggests a dipole interpretation. Indeed, the rigorous aspects of this can be recognized by direct inspection of Eq. (S6): for general interfaces, $\partial\Omega$ with outward surface normal $\hat{\mathbf{n}}$, this motivates the association of the physical role of $d_\perp$ with a dipole density $\mathbf{P}(\mathbf{r}) \equiv \boldsymbol{\pi}(\mathbf{r})\delta_{\partial\Omega}(\mathbf{r})$, expressed in terms of a surface dipole density $\boldsymbol{\pi}(\mathbf{r}) \equiv d_\perp\sigma(\mathbf{r})\hat{\mathbf{n}}$ proportional to the classical surface charge $\sigma(\mathbf{r})$ and a surface Dirac delta function $\delta_{\partial\Omega}(\mathbf{r})$.[4] Curiously, this useful very interpretation appears not to have been emphasized until recently, when it was noted and utilized in a computational scheme by Yan *et al.* [S6].

The deduction of a similar interpretation of $d_\parallel$ is less obvious. Nevertheless, a connection can be discerned by comparing Eq. (S15a) at $d_\perp = 0$, i.e. $r = -\frac{\varepsilon_\mathrm{m}-\varepsilon_\mathrm{d}+(\varepsilon_\mathrm{m}-\varepsilon_\mathrm{d})kd_\parallel}{\varepsilon_\mathrm{m}+\varepsilon_\mathrm{d}+(\varepsilon_\mathrm{m}-\varepsilon_\mathrm{d})kd_\parallel}$, to the nonretarded reflection coefficient of a planar interface supporting a surface current due to a finite surface conductivity $s$, reading $r = -\frac{\varepsilon_\mathrm{m}-\varepsilon_\mathrm{d}+g}{\varepsilon_\mathrm{m}+\varepsilon_\mathrm{d}+g}$ with $g \equiv \mathrm{i}sk/\varepsilon_0\omega$ [S7]. Comparison of the two expressions then demonstrates that the impact of $d_\parallel$ is equivalent to the existence of a surface current $\mathbf{K}(\mathbf{r}) = s\mathbf{E}_\parallel(\mathbf{r})$, driven by the tangential components of the

[4] The surface Dirac delta function is formally via the indicator function $1_\Omega(\mathbf{r}) \equiv \begin{cases} 1, \text{if } \mathbf{r}\in\Omega \\ 0, \text{if } \mathbf{r}\notin\Omega \end{cases}$ of the enclosed region $\Omega$, through its outward normal derivative $\delta_{\partial\Omega}(\mathbf{r}) \equiv \hat{\mathbf{n}} \cdot \boldsymbol{\nabla} 1_\Omega(\mathbf{r})$.

total electric field $\mathbf{E}_\parallel$, provided the surface conductivity is chosen as $s \equiv \mathrm{i}\varepsilon_0\omega(\varepsilon_\mathrm{d} - \varepsilon_\mathrm{m})d_\parallel$.[5] To the best of our knowledge, this interpretation seems not to have been noted previously.

In summary, the influence of $d_\perp$ and $d_\parallel$ at a general interface $\partial\Omega$ can be included by allowing a finite surface dipole and current density, $\boldsymbol{\pi}(\mathbf{r}) = d_\perp\sigma(\mathbf{r})\hat{\mathbf{n}}$ and $\mathbf{K}(\mathbf{r}) = \mathrm{i}\varepsilon_0\omega(\varepsilon_\mathrm{d} - \varepsilon_\mathrm{m})d_\parallel\mathbf{E}_\parallel(\mathbf{r})$, respectively. Such a treatment is equivalent and consistent with that leading to Eqs. (S15). The interpretation is clearly highly useful because it allows the direct introduction of the $d$-parameters in existing electrodynamic computational schemes by adopting BCs which allow the existence of $\boldsymbol{\pi}(\mathbf{r})$ and $\mathbf{K}(\mathbf{r})$.

### B. Reformulating the $d_\parallel$-parameter

The definition of $d_\parallel$ given in Eq. (S12) explicitly refers to the asymptotic currents; for many purposes, a reformulation is preferable such that only the real, quantum mechanical currents are referenced. This is the purpose of this section: demonstrate the equivalence of Eqs. (S12) and Eq. (1) of the main text. We note immediately, that the equivalence is achievable only in the small wavevector limit, i.e. for $k \ll |x_{1,2}^{-1}|$. This reduction does not pose any real restriction, since such an approximation is consistent with our overall aim of formulating a leading-order accurate scheme; the $k$-dependence of $d_\parallel$ is ignored regardless.

In the $k \ll |x_{1,2}^{-1}|$ limit, the classical asymptotic current $\mathrm{J}_y^\infty(x)$ does not change appreciably over the region $x \in [x_1, x_2]$. This allows the following series of reductions:

$$\begin{aligned}
d_\parallel &= \frac{\int_{x_1}^{x_2}\left[\mathrm{J}_y(x) - \mathrm{J}_y^\infty(x)\right]\,\mathrm{d}x}{\mathrm{J}_y^\infty(0^-) - \mathrm{J}_y^\infty(0^+)} \\
&\overset{k\ll|x_{1,2}^{-1}|}{\simeq} \frac{\int_{x_1}^{x_2}\mathrm{J}_y(x)\,\mathrm{d}x + x_1\mathrm{J}_y^\infty(x_1) - x_2\mathrm{J}_y^\infty(x_2)}{\mathrm{J}_y^\infty(x_1) - \mathrm{J}_y^\infty(x_2)} \\
&= \frac{\int_{x_1}^{x_2}\mathrm{J}_y(x)\,\mathrm{d}x + x_1\mathrm{J}_y(x_1) - x_2\mathrm{J}_y(x_2)}{\mathrm{J}_y(x_1) - \mathrm{J}_y(x_2)} \\
&= \frac{\int_{x_1}^{x_2}\mathrm{J}_y(x)\,\mathrm{d}x - \int_{x_1}^{x_2}\frac{\partial}{\partial x}\left[x\mathrm{J}_y(x)\right]\mathrm{d}x}{-\int_{x_1}^{x_2}\frac{\partial\mathrm{J}_y(x)}{\partial x}\,\mathrm{d}x} \\
&= \frac{\int_{x_1}^{x_2} x\frac{\partial\mathrm{J}_y(x)}{\partial x}\,\mathrm{d}x}{\int_{x_1}^{x_2}\frac{\partial\mathrm{J}_y(x)}{\partial x}\,\mathrm{d}x},
\end{aligned} \tag{S16}$$

where, at the third equality, it has been used that $\mathrm{J}_y^\infty(x) = \mathrm{J}_y(x)$ for $x \geq |x_{1,2}|$ cf. the definition of the asymptotic quantities. Finally, Eq. (1) is recovered by noting that contributions for $x > |x_{1,2}|$ are negligible by the assumption of surface localization, i.e. the integration domain may be extended to $x \in ]-\infty, \infty[$.

## II. A GENERALIZED NONRETARDED BOUNDARY INTEGRAL EQUATION

In this section, we derive the generalized nonretarded boundary integral equation (nBIE) presented in Eqs. (2) of the main text. For purposes of clarity, we split the derivation such that we initially consider effects only due to $d_\perp$ – and only afterwards include $d_\parallel$ in the derivation.

---

[5] An alternate approach to this identification origins from the definition of $d_\parallel$, i.e. from Eq. (S12). Specifically, in the low-$k$ limit (in the spirit of Section I.B) the denominator may be approximated by $\mathrm{J}_y^\infty(0^-) - \mathrm{J}_y^\infty(0^+) = -\mathrm{i}\varepsilon_0(\varepsilon_\mathrm{m} - 1)\mathrm{E}_y^\infty(0^-) + \mathrm{i}\varepsilon_0(\varepsilon_\mathrm{d} - 1)\mathrm{E}_y^\infty(0^+)] \simeq \mathrm{i}\varepsilon_0\omega(\varepsilon_\mathrm{d} - \varepsilon_\mathrm{m})\mathrm{E}_y^\infty(0)$, since $\mathrm{E}_y^\infty(x)$ is approximately constant over $x \ll |x_{1,2}|$ in the low-$k$ limit. The conductivity $s$ is introduced as the coefficient of an equivalent boundary current driven by the classical asymptotic field $\mathrm{E}_y^\infty(0)$, whose value equals the numerator of Eq. (S12); i.e. $s\mathrm{E}_y^\infty(0)$ is the nonclassical contribution to the integrated quantum mechanical current $\mathrm{J}_y(x)$ in the sense $s\mathrm{E}_y^\infty(0) \equiv \int_{x_1}^{x_2}\left[\mathrm{J}_y(x) - \mathrm{J}_y^\infty(x)\right]\mathrm{d}x$. Combined with the definition of $d_\parallel$ this then demonstrates that $s = \mathrm{i}\varepsilon_0(\varepsilon_\mathrm{d} - \varepsilon_\mathrm{m})d_\parallel$.

### A. The perpendicular Feibelman parameter: surface dipole density

To derive the nBIE for an arbitrary plasmonic system, we first write down the expression for the total electric potential $\phi(\mathbf{r})$ due to a set of surface charge and dipole densities, $\sigma(\mathbf{r})$ and $\boldsymbol{\pi}(\mathbf{r})$, in vacuum [S8]

$$\phi(\mathbf{r}) = \phi^{\text{ext}}(\mathbf{r}) + \frac{1}{4\pi\varepsilon_0}\int_{\partial\Omega} g(\mathbf{r},\mathbf{r}')\sigma(\mathbf{r}')\,\mathrm{d}^2\mathbf{r}' + \frac{1}{4\pi\varepsilon_0}\int_{\partial\Omega}\big[\boldsymbol{\nabla}' g(\mathbf{r},\mathbf{r}')\big]\cdot\boldsymbol{\pi}(\mathbf{r}')\,\mathrm{d}^2\mathbf{r}', \tag{S17}$$

with external potential $\phi^{\text{ext}}(\mathbf{r})$, Coulomb interaction $g(\mathbf{r},\mathbf{r}') = 1/|\mathbf{r}-\mathbf{r}'|$, and (not necessarily connected) boundary region $\partial\Omega$ separating a metallic ($\varepsilon_\text{m}$) interior from a dielectric ($\varepsilon_\text{d}$) exterior. The dipole density is related to the charge density and $d_\perp$ through $\boldsymbol{\pi}(\mathbf{r}') = d_\perp\sigma(\mathbf{r}')\hat{\mathbf{n}}'$, cf. Section I.A.

The potential and charge density are interrelated by the Poisson equation, which, when integrated over a pillbox enclosing an element $\mathbf{r}\in\partial\Omega$, dictates that

$$\begin{aligned}\sigma(\mathbf{r}) &= -\varepsilon_0 \lim_{\delta\to 0^+}\big[\hat{\mathbf{n}}\cdot\boldsymbol{\nabla}\phi(\mathbf{r}+\delta\hat{\mathbf{n}}) - \hat{\mathbf{n}}\cdot\boldsymbol{\nabla}\phi(\mathbf{r}-\delta\hat{\mathbf{n}})\big]\\ &= \varepsilon_0\frac{\varepsilon_\text{d}-\varepsilon_\text{m}}{\varepsilon_\text{m}}\lim_{\delta\to 0^+}\big[\hat{\mathbf{n}}\cdot\boldsymbol{\nabla}\phi(\mathbf{r}+\delta\hat{\mathbf{n}})\big],\end{aligned} \tag{S18}$$

where $\phi(\mathbf{r}\pm\delta\hat{\mathbf{n}})$ represent the potentials along the boundary in the dielectric and metallic regions, respectively. The second line of the equation is obtained by using the BC for the continuity across $\partial\Omega$ of the normal components of the **D**-field. By applying an operation $\hat{\mathbf{n}}\cdot\boldsymbol{\nabla}$ onto Eq. (S17) at a point just outside the boundary, i.e. at $\mathbf{r}+\delta\hat{\mathbf{n}}$, while making use of Eq. (S18), we then obtain

$$\begin{aligned}4\pi\frac{\varepsilon_\text{m}}{\varepsilon_\text{d}-\varepsilon_\text{m}}\sigma(\mathbf{r}) &= 4\pi\varepsilon_0[\hat{\mathbf{n}}\cdot\boldsymbol{\nabla}\phi^{\text{ext}}(\mathbf{r})]\\ &\quad+\lim_{\delta\to 0^+}\int_{\partial\Omega}\hat{\mathbf{n}}\cdot\boldsymbol{\nabla} g(\mathbf{r}+\delta\hat{\mathbf{n}},\mathbf{r}')\sigma(\mathbf{r}')\,\mathrm{d}^2\mathbf{r}'\\ &\quad+d_\perp\lim_{\delta\to 0^+}\int_{\partial\Omega}\big[\hat{\mathbf{n}}\cdot\boldsymbol{\nabla}\boldsymbol{\nabla}' g(\mathbf{r}+\delta\hat{\mathbf{n}},\mathbf{r}')\cdot\hat{\mathbf{n}}'\big]\sigma(\mathbf{r}')\,\mathrm{d}^2\mathbf{r}'.\end{aligned} \tag{S19}$$

A singular contribution at $\lim_{\delta\to 0^+}(\mathbf{r}+\delta\hat{\mathbf{n}}) = \mathbf{r}'$ can be extracted from the first integral term by using the identity $\lim_{\delta\to 0^+}\hat{\mathbf{n}}\cdot\boldsymbol{\nabla} g(\mathbf{r}+\delta\hat{\mathbf{n}},\mathbf{r}') = \mathcal{P}[\hat{\mathbf{n}}\cdot\boldsymbol{\nabla} g(\mathbf{r},\mathbf{r}')] - 2\pi\delta(\mathbf{r}-\mathbf{r}')$, allowing a final reduction, such that

$$\Lambda\sigma(\mathbf{r}) = \sigma^{\text{ext}}(\mathbf{r}) + \mathcal{P}\int_{\partial\Omega}\hat{\mathbf{n}}\cdot\boldsymbol{\nabla} g(\mathbf{r},\mathbf{r}')\sigma(\mathbf{r}')\,\mathrm{d}^2\mathbf{r}' + d_\perp\lim_{\delta\to 0^+}\int_{\partial\Omega}\big[\hat{\mathbf{n}}\cdot\boldsymbol{\nabla}\boldsymbol{\nabla}' g(\mathbf{r}+\delta\hat{\mathbf{n}},\mathbf{r}')\cdot\hat{\mathbf{n}}'\big]\sigma(\mathbf{r}')\,\mathrm{d}^2\mathbf{r}', \tag{S20a}$$

with external perturbation $\sigma^{\text{ext}}(\mathbf{r}) \equiv 4\pi\varepsilon_0[\hat{\mathbf{n}}\cdot\boldsymbol{\nabla}\phi^{\text{ext}}(\mathbf{r})]$. The system constitutes a boundary integral equation in the self-consistent charge density $\sigma(\mathbf{r})$. The prefactor $\Lambda$ is an eigenvalue in the absence of external perturbations, and is defined by

$$\Lambda \equiv 2\pi\frac{\varepsilon_\text{d}+\varepsilon_\text{m}}{\varepsilon_\text{d}-\varepsilon_\text{m}}. \tag{S20b}$$

### B. The parallel Feibelman parameter: surface current density

Generalizing the above nBIE to account also for $d_\parallel$ is achieved by allowing a surface current contribution $\mathbf{K}(\mathbf{r}) = s[-\boldsymbol{\nabla}_\parallel\phi(\mathbf{r})]$, see Section I.A, with surface conductivity $s \equiv \mathrm{i}\varepsilon_0\omega(\varepsilon_\text{d}-\varepsilon_\text{m})d_\parallel$ and tangential gradient $\boldsymbol{\nabla}_\parallel$ defined by $\boldsymbol{\nabla}_\parallel = \mathbf{I}_\parallel\boldsymbol{\nabla}$ via $\mathbf{I}_\parallel = \mathbf{I} - \hat{\mathbf{n}}\hat{\mathbf{n}}$. The most direct path to including it self-consistently in the nBIE lies in recognizing that the surface-current $\mathbf{K}$ modifies the BC used in reducing Eq. (S18). Specifically, the **D**-field normal components develop a discontinuity $\lim_{\delta\to 0^+}\big\{\hat{\mathbf{n}}\cdot\big[\mathbf{D}(\mathbf{r}+\delta\hat{\mathbf{n}}) - \mathbf{D}(\mathbf{r}-\delta\hat{\mathbf{n}})\big]\big\} = \sigma_\mathbf{K}(\mathbf{r})$ equal to the surface density associated with $\mathbf{K}$, equaling $\sigma_\mathbf{K}(\mathbf{r}) = \mathrm{i}\omega^{-1}\boldsymbol{\nabla}_\parallel\cdot\mathbf{K}(\mathbf{r})$. In turn, this modifies Eq. (S18), which generalizes to

$$\begin{aligned}\sigma(\mathbf{r}) &= -\varepsilon_0\lim_{\delta\to 0^+}\big[\hat{\mathbf{n}}\cdot\boldsymbol{\nabla}\phi(\mathbf{r}+\delta\hat{\mathbf{n}}) - \hat{\mathbf{n}}\cdot\boldsymbol{\nabla}\phi(\mathbf{r}-\delta\hat{\mathbf{n}})\big]\\ &= \varepsilon_0\frac{\varepsilon_\text{d}-\varepsilon_\text{m}}{\varepsilon_\text{m}}\Big\{\lim_{\delta\to 0^+}\big[\hat{\mathbf{n}}\cdot\boldsymbol{\nabla}\phi(\mathbf{r}+\delta\hat{\mathbf{n}})\big] - d_\parallel\nabla_\parallel^2\phi(\mathbf{r})\Big\},\end{aligned} \tag{S21}$$

for points $\mathbf{r} \in \partial\Omega$. The reasoning leading to Eq. (S19) is then similarly modified (omitting $\phi^{\text{ext}}$ for brevity):

$$4\pi \frac{\varepsilon_\text{m}}{\varepsilon_\text{d} - \varepsilon_\text{m}} \sigma(\mathbf{r}) = \lim_{\delta \to 0^+} \int_{\partial\Omega} \hat{\mathbf{n}} \cdot \nabla g(\mathbf{r} + \delta\hat{\mathbf{n}}, \mathbf{r}')\sigma(\mathbf{r}')\, \mathrm{d}^2\mathbf{r}' \\ + d_\perp \lim_{\delta \to 0^+} \int_{\partial\Omega} \big[\hat{\mathbf{n}} \cdot \nabla\nabla' g(\mathbf{r} + \delta\hat{\mathbf{n}}, \mathbf{r}') \cdot \hat{\mathbf{n}}'\big]\sigma(\mathbf{r}')\, \mathrm{d}^2\mathbf{r}' \\ - 4\pi\varepsilon_0 d_\parallel \nabla_\parallel^2 \phi(\mathbf{r}), \tag{S22}$$

which, after extraction of the singularity in the first integral term and substitution of $\phi(\mathbf{r})$ via Eq. (S17) finally produces

$$\Lambda\sigma(\mathbf{r}) = \mathcal{P}\int_{\partial\Omega} \hat{\mathbf{n}} \cdot \nabla g(\mathbf{r}, \mathbf{r}')\sigma(\mathbf{r}')\, \mathrm{d}^2\mathbf{r}' + d_\perp \lim_{\delta \to 0^+} \int_{\partial\Omega} \big[\hat{\mathbf{n}} \cdot \nabla\nabla' g(\mathbf{r} + \delta\hat{\mathbf{n}}, \mathbf{r}') \cdot \hat{\mathbf{n}}'\big]\sigma(\mathbf{r}')\, \mathrm{d}^2\mathbf{r}' \\ - d_\parallel \int_{\partial\Omega} \nabla_\parallel^2 g(\mathbf{r}, \mathbf{r}')\sigma(\mathbf{r}')\, \mathrm{d}^2\mathbf{r}', \tag{S23}$$

where a cross-term of order $O(d_\perp d_\parallel)$ has been dropped, consistent with our aim of attaining a first-order accurate scheme [and, in addition, consistent with the conventional planar Feibelman approach where an equivalent cross-term is dropped as well, see Eq. (S15)]. This is the modified nBIE given in Eq. (3a) of the main text.

## III. DERIVATION OF PERTURBATION RESULTS

In this section, we derive the simplified forms of the perturbation factors $\Lambda_\perp^{(1)}$ and $\Lambda_\parallel^{(1)}$ given in Eqs. (3b) and (3c) of the main text. The derivations involve the eigensolutions of the classical nBIE [which follow from the classical truncation, i.e. $d_\perp = d_\parallel = 0$, of Eq. (S23)], which we here define for future reference:

$$\Lambda_n^{(0)}|\sigma_n^{(0)}\rangle = \mathsf{K}|\sigma_n^{(0)}\rangle \quad \text{with coordinate form} \quad \Lambda_n^{(0)}\sigma_n^{(0)}(\mathbf{r}) = \mathcal{P}\int_{\partial\Omega} \hat{\mathbf{n}} \cdot \nabla g(\mathbf{r}, \mathbf{r}')\sigma_n^{(0)}(\mathbf{r}')\, \mathrm{d}^2\mathbf{r}', \tag{S24a}$$

with the eigenindex $n$ indicated explicitly. Similarly, we define its biorthogonal partner by the associated surface potential $\phi_n^{(0)}(\mathbf{r})$ which relates to $\sigma_n^{(0)}(\mathbf{r})$ through the classical truncation of Eq. (S17)

$$|\phi_n^{(0)}\rangle = \frac{1}{4\pi\varepsilon_0}\mathsf{g}|\sigma_n^{(0)}\rangle \quad \text{with coordinate form} \quad \phi_0^n(\mathbf{r}) = \frac{1}{4\pi\varepsilon_0}\int_{\partial\Omega} g(\mathbf{r}, \mathbf{r}')\sigma_0^n(\mathbf{r}')\, \mathrm{d}^2\mathbf{r}'. \tag{S24b}$$

In the following, we omit explicit reference to the eigenindex $n$; its presence remains implicitly understood.

### A. Perpendicular component

The perpendicular perturbation factor $\Lambda_\perp^{(1)}$ associated with $d_\perp$ is given by standard perturbation theory adapted to a biorthogonal basis, such that[6]

$$\Lambda_\perp^{(1)} \equiv \frac{\langle\phi^{(0)}|\mathsf{V}_\perp|\sigma^{(0)}\rangle}{\langle\phi^{(0)}|\sigma^{(0)}\rangle} = \frac{\lim_{\delta\to 0^+} \int_{\partial\Omega}\int_{\partial\Omega} \overline{\phi^{(0)}(\mathbf{r})}\big[\hat{\mathbf{n}} \cdot \nabla\nabla' g(\mathbf{r} + \delta\hat{\mathbf{n}}, \mathbf{r}') \cdot \hat{\mathbf{n}}'\big]\sigma^{(0)}(\mathbf{r}')\, \mathrm{d}^2\mathbf{r}\, \mathrm{d}^2\mathbf{r}'}{\int_{\partial\Omega} \overline{\phi^{(0)}(\mathbf{r})}\sigma^{(0)}(\mathbf{r})\, \mathrm{d}^2\mathbf{r}}, \tag{S25}$$

---

[6] Though it is in principle possible to choose the classical basis functions as entirely real [S9], we retain a complex notation since it is often more useful for practical calculations.

which is just the coordinate expansion obtained from the explicit form of $\mathsf{V}_\perp$. The result can be significantly simplified: specifically, writing the correction as a fraction $\Lambda_\perp^{(1)} \equiv \mathcal{N}_\perp/\mathcal{D}_\perp$ we simplify the numerator $\mathcal{N}_\perp$

$$\begin{aligned}
\mathcal{N}_\perp &\equiv \lim_{\delta\to 0^+}\int_{\partial\Omega}\int_{\partial\Omega}\overline{\phi^{(0)}(\mathbf{r})}[\hat{\mathbf{n}}\cdot\boldsymbol{\nabla}\boldsymbol{\nabla}'g(\mathbf{r}+\delta\hat{\mathbf{n}},\mathbf{r}')\cdot\hat{\mathbf{n}}']\sigma^{(0)}(\mathbf{r}')\,\mathrm{d}^2\mathbf{r}\,\mathrm{d}^2\mathbf{r}' \\
&\stackrel{a}{=} \lim_{\delta\to 0^+}\int_{\partial\Omega}\boldsymbol{\nabla}'\bigg\{\int_{\partial\Omega}\hat{\mathbf{n}}\cdot\big[\overline{\phi^{(0)}(\mathbf{r})}\boldsymbol{\nabla}g(\mathbf{r}+\delta\hat{\mathbf{n}},\mathbf{r}')\big]\,\mathrm{d}^2\mathbf{r}\bigg\}\cdot\hat{\mathbf{n}}'\sigma^{(0)}(\mathbf{r}')\,\mathrm{d}^2\mathbf{r}' \\
&\stackrel{b}{=} \lim_{\delta\to 0^+}\int_{\partial\Omega}\boldsymbol{\nabla}'\bigg\{\int_{\partial\Omega_\delta^+}\hat{\mathbf{n}}\cdot\big[\overline{\phi^{(0)}(\mathbf{r})}\boldsymbol{\nabla}g(\mathbf{r},\mathbf{r}')\big]\,\mathrm{d}^2\mathbf{r}\bigg\}\cdot\hat{\mathbf{n}}'\sigma^{(0)}(\mathbf{r}')\,\mathrm{d}^2\mathbf{r}' \\
&\stackrel{c}{=} \lim_{\delta\to 0^+}\int_{\partial\Omega}\boldsymbol{\nabla}'\bigg\{-\int_{\mathbb{R}^3\setminus\Omega_\delta^+}\boldsymbol{\nabla}\cdot\big[\overline{\phi^{(0)}(\mathbf{r})}\boldsymbol{\nabla}g(\mathbf{r},\mathbf{r}')\big]\,\mathrm{d}^3\mathbf{r}\bigg\}\cdot\hat{\mathbf{n}}'\sigma^{(0)}(\mathbf{r}')\,\mathrm{d}^2\mathbf{r}' \\
&\stackrel{d}{=} \lim_{\delta\to 0^+}\int_{\partial\Omega}\boldsymbol{\nabla}'\bigg\{-\int_{\mathbb{R}^3\setminus\Omega_\delta^+}\boldsymbol{\nabla}\cdot\big[g(\mathbf{r},\mathbf{r}')\boldsymbol{\nabla}\overline{\phi^{(0)}(\mathbf{r})}\big]\,\mathrm{d}^3\mathbf{r}\bigg\}\cdot\hat{\mathbf{n}}'\sigma^{(0)}(\mathbf{r}')\,\mathrm{d}^2\mathbf{r}' \\
&\stackrel{e}{=} \lim_{\delta\to 0^+}\int_{\partial\Omega}\boldsymbol{\nabla}'\bigg\{\int_{\partial\Omega_\delta^+}\hat{\mathbf{n}}\cdot\big[g(\mathbf{r},\mathbf{r}')\boldsymbol{\nabla}\overline{\phi^{(0)}(\mathbf{r})}\big]\,\mathrm{d}^2\mathbf{r}\bigg\}\cdot\hat{\mathbf{n}}'\sigma^{(0)}(\mathbf{r}')\,\mathrm{d}^2\mathbf{r}' \\
&\stackrel{f}{=} \lim_{\delta\to 0^+}\int_{\partial\Omega}\bigg\{\int_{\partial\Omega}\big[\hat{\mathbf{n}}'\cdot\boldsymbol{\nabla}'g(\mathbf{r}+\delta\hat{\mathbf{n}},\mathbf{r}')\big]\big[\hat{\mathbf{n}}\cdot\boldsymbol{\nabla}\overline{\phi^{(0)}(\mathbf{r}+\delta\hat{\mathbf{n}})}\big]\,\mathrm{d}^2\mathbf{r}\bigg\}\sigma^{(0)}(\mathbf{r}')\,\mathrm{d}^2\mathbf{r}' \\
&\stackrel{g}{=} \frac{\Lambda^{(0)}-2\pi}{4\pi\varepsilon_0}\int_{\partial\Omega}\bigg\{\mathcal{P}\int_{\partial\Omega}\big[\hat{\mathbf{n}}'\cdot\boldsymbol{\nabla}'g(\mathbf{r},\mathbf{r}')+2\pi\delta(\mathbf{r}-\mathbf{r}')\big]\,\overline{\sigma^{(0)}(\mathbf{r})}\,\mathrm{d}^2\mathbf{r}\bigg\}\sigma^{(0)}(\mathbf{r}')\,\mathrm{d}^2\mathbf{r}' \\
&\stackrel{h}{=} \frac{(\Lambda^{(0)}-2\pi)(\Lambda^{(0)}+2\pi)}{4\pi\varepsilon_0}\int_{\partial\Omega}|\sigma^{(0)}(\mathbf{r}')|^2\,\mathrm{d}^2\mathbf{r}',
\end{aligned} \tag{S26}$$

with the following steps:

*a*. Rearrangement of $\mathbf{r}$- and $\mathbf{r}'$-dependent terms.

*b*. Coordinate transformation $\mathbf{r}'' = \mathbf{r} + \delta\hat{\mathbf{n}}$, changing the integration boundary to $\partial\Omega_\delta^+$ (denoting the $\delta\hat{\mathbf{n}}$-enlarged correspondent of $\partial\Omega$). The transformation leaves the argument of $\phi^{(0)}(\mathbf{r})$ unchanged in the $\delta \to 0^+$ limit, cf. continuity of the potential. Primed distinction is dropped immediately.

*c*. Application of the divergence theorem to the complement of $\Omega_\delta^+$, i.e. to $\mathbf{r} \in \mathbb{R}^3\setminus\Omega_\delta^+$.

*d*. The term $\boldsymbol{\nabla}\cdot[\overline{\phi^{(0)}(\mathbf{r})}\boldsymbol{\nabla}g(\mathbf{r},\mathbf{r}')]$ is rewritten as $\boldsymbol{\nabla}\cdot[g(\mathbf{r},\mathbf{r}')\boldsymbol{\nabla}\overline{\phi^{(0)}(\mathbf{r})}] - g(\mathbf{r},\mathbf{r}')\nabla^2\overline{\phi^{(0)}(\mathbf{r})} + \overline{\phi^{(0)}(\mathbf{r})}\nabla^2 g(\mathbf{r},\mathbf{r}')$. The last two terms in this expression do not contribute to the integral: specifically, $\nabla^2\overline{\phi^{(0)}(\mathbf{r})}$ is nonzero only for $\mathbf{r} \in \partial\Omega$ cf. the Poisson equation but $\mathbf{r} \in \mathbb{R}^3\setminus\Omega_\delta^+$ does not contain $\partial\Omega$ – similarly, $\nabla^2 g(\mathbf{r},\mathbf{r}') = -4\pi\delta(\mathbf{r}-\mathbf{r}')$ but the $\mathbf{r}$- and $\mathbf{r}'$ integration domains do not overlap.

*e*. Application of the divergence theorem.

*f*. Rearrangement of terms and inversion of the coordinate transformation of step *b*.

*g*. The first square bracketed term is reduced via the relation $\lim_{\delta\to 0^+}\int_{\partial\Omega}\hat{\mathbf{n}}'\cdot\boldsymbol{\nabla}'g(\mathbf{r}+\delta\hat{\mathbf{n}},\mathbf{r}')f(\mathbf{r})\,\mathrm{d}^2\mathbf{r} = \mathcal{P}\int_{\partial\Omega}\hat{\mathbf{n}}'\cdot\boldsymbol{\nabla}'g(\mathbf{r},\mathbf{r}')f(\mathbf{r})\,\mathrm{d}^2\mathbf{r} + 2\pi f(\mathbf{r}')$ (for smooth test functions $f$), while the second bracketed term is converted via Eq. (S18).

*h*. Besides a trivial reduction of the Dirac delta term, the remaining $\mathbf{r}$ integral is reduced via Eq. (S24a).

Accordingly, the entire perturbation factor is reduced to the result provided in Eq. (3b), i.e. to

$$\Lambda_\perp^{(1)} = \frac{(\Lambda^{(0)})^2-(2\pi)^2}{4\pi\varepsilon_0}\frac{\langle\sigma^{(0)}|\sigma^{(0)}\rangle}{\langle\phi^{(0)}|\sigma^{(0)}\rangle}. \tag{S27}$$

### B. Parallel component

The $\Lambda_\parallel^{(1)}$ perturbation parameter may be reduced in much the same way as its perpendicular correspondent. Its explicit form is obtained by expanding the $\mathsf{V}_\parallel$ into its coordinate representation, such that

$$\Lambda_\parallel^{(1)} \equiv \frac{\langle\phi^{(0)}|\mathsf{V}_\parallel|\sigma^{(0)}\rangle}{\langle\phi^{(0)}|\sigma^{(0)}\rangle} = -\frac{\int_{\partial\Omega}\int_{\partial\Omega}\overline{\phi^{(0)}(\mathbf{r})}\nabla_\parallel^2 g(\mathbf{r},\mathbf{r}')\sigma^{(0)}(\mathbf{r}')\,\mathrm{d}^2\mathbf{r}\,\mathrm{d}^2\mathbf{r}'}{\int_{\partial\Omega}\overline{\phi^{(0)}(\mathbf{r})}\sigma^{(0)}(\mathbf{r})\,\mathrm{d}^2\mathbf{r}}, \tag{S28}$$

The numerator, $\mathcal{N}_\parallel$, of this expression is then reduced according to

$$\begin{aligned}\mathcal{N}_\parallel &\equiv -\int_{\partial\Omega}\int_{\partial\Omega} \overline{\phi^{(0)}(\mathbf{r})}\nabla_\parallel^2 g(\mathbf{r},\mathbf{r}')\sigma^{(0)}(\mathbf{r}')\,\mathrm{d}^2\mathbf{r}\,\mathrm{d}^2\mathbf{r}' \\ &\overset{\mathrm{a}}{=} -4\pi\varepsilon_0 \int_{\partial\Omega} \overline{\phi^{(0)}(\mathbf{r})}\nabla_\parallel^2\phi^{(0)}(\mathbf{r})\,\mathrm{d}^2\mathbf{r} \\ &\overset{\mathrm{b}}{=} 4\pi\varepsilon_0 \int_{\partial\Omega} \big[\boldsymbol{\nabla}_\parallel\overline{\phi^{(0)}(\mathbf{r})}\big]\cdot\big[\boldsymbol{\nabla}_\parallel\phi^{(0)}(\mathbf{r})\big]\,\mathrm{d}^2\mathbf{r},\end{aligned} \tag{S29}$$

whose steps are more modest than its perpendicular equivalent:

*a*. The $\mathbf{r}'$ integral is reduced directly through Eq. (S24b).

*b*. The term $\overline{\phi^{(0)}(\mathbf{r})}\nabla_\parallel^2\phi^{(0)}(\mathbf{r})$ is rewritten as $\boldsymbol{\nabla}_\parallel\cdot\big[\overline{\phi^{(0)}(\mathbf{r})}\boldsymbol{\nabla}_\parallel\phi^{(0)}(\mathbf{r})\big] - \big[\boldsymbol{\nabla}_\parallel\overline{\phi^{(0)}(\mathbf{r})}\big]\cdot\big[\boldsymbol{\nabla}_\parallel\phi^{(0)}(\mathbf{r})\big]$. The former term does not contribute to the integral cf. the surface divergence theorem:[7] since $\partial\Omega$ is a closed surface its periphery vanishes, zeroing its integral as well.

The result given in Eq. (3c) of the main text is consequently retrieved, such that

$$\Lambda_\parallel^{(1)} = 4\pi\varepsilon_0 \frac{\langle\boldsymbol{\nabla}_\parallel\phi^{(0)}|\boldsymbol{\nabla}_\parallel\phi^{(0)}\rangle}{\langle\phi^{(0)}|\sigma^{(0)}\rangle}. \tag{S30}$$

## IV. POSITIVE AND NEGATIVE DEFINITENESS OF NONCLASSICAL PERTURBATION FACTORS

Here, we prove that $\Lambda_\perp^{(1)}$ and $\Lambda_\parallel^{(1)}$, as defined by Eqs. (S26) and (S30), are negative and positive definite functions, respectively, of the classical eigensolutions $\{\Lambda^{(0)}, |\sigma^{(0)}\rangle, |\phi^{(0)}\rangle\}$, in the sense that $\Lambda_\perp^{(1)} < 0$ and $\Lambda_\parallel^{(1)} > 0$ for nontrivial eigensolutions.

Before specializing to either, we note that $\Lambda_\alpha^{(1)} \propto 1/\langle\phi^{(0)}|\sigma^{(0)}\rangle$. Notably, $\langle\phi|\sigma\rangle$ is positive for all nonzero states: $\langle\phi|\sigma\rangle = (4\pi\varepsilon_0)^{-1}\langle\sigma|\mathsf{g}|\sigma\rangle = (4\pi\varepsilon_0)^{-1}\int_{\partial\Omega}\int_{\partial\Omega} g(\mathbf{r},\mathbf{r}')\overline{\sigma(\mathbf{r}')}\sigma(\mathbf{r})\,\mathrm{d}^2\mathbf{r}'\mathrm{d}^2\mathbf{r} > 0$ since the Coulomb operator $\mathsf{g}$, with elements $g(\mathbf{r},\mathbf{r}') \equiv |\mathbf{r}-\mathbf{r}'|^{-1}$, is a symmetric, positive definite operator [S9]. Accordingly, $\langle\phi^{(0)}|\sigma^{(0)}\rangle > 0$ for nontrivial states, and it is sufficient to consider the numerator of Eqs. (S26) and (S30).

Considering first the numerator of $\Lambda_\perp^{(1)}$, Eq. (S26): $\langle\phi^{(0)}|\mathsf{V}_\perp|\sigma^{(0)}\rangle = (4\pi\varepsilon_0)^{-1}\langle\sigma^{(0)}|\sigma^{(0)}\rangle[(\Lambda^{(0)})^2 - (2\pi)^2]$. Since $\langle\sigma^{(0)}|\sigma^{(0)}\rangle > 0$ for all nonzero states, it follows that $\Lambda_\perp^{(1)}$ is negative definite iff $(\Lambda^{(0)})^2 - (2\pi)^2 < 0$ for all classical eigensolutions. Fortunately, the nontrivial eigenvalues of $\mathsf{K}$ are real and restricted to the domain $|\Lambda^{(0)}| < 2\pi$, as shown in Ref. S10.[8] This completes the proof for the negative definiteness of $\Lambda_\perp^{(1)}$.

Next, we consider $\Lambda_\parallel^{(1)}$ of Eq. (S30). Its numerator is simply $\langle\phi^{(0)}|\mathsf{V}_\perp|\sigma^{(0)}\rangle = 4\pi\varepsilon_0\langle\boldsymbol{\nabla}_\parallel\phi^{(0)}|\boldsymbol{\nabla}_\parallel\phi^{(0)}\rangle$. It immediately follows that this is a positive quantity for non-uniform potentials (by choice, we categorize uniform/constant solutions as trivial): by the above arguments $\Lambda_\parallel^{(1)}$ is consequently positive definite.

A more general question is whether the nonclassical operator $\mathsf{V}_\perp$ is a negative definite operator as well, in the sense $\langle\phi|\mathsf{V}_\perp|\sigma\rangle/\langle\phi|\sigma\rangle < 0$ for all partners $\{|\sigma\rangle, |\phi\rangle\}$ (and, similarly, is $\mathsf{V}_\parallel$ positive definite in the sense $\langle\phi|\mathsf{V}_\parallel|\sigma\rangle/\langle\phi|\sigma\rangle > 0$)? That question is left unanswered by these considerations, which only demonstrate that the operator's diagonal elements, viewed in the classical eigenbasis, are negative (positive) definite.

---

[7] This theorem is a variant of Stokes theorem, and reads: $\int_S \boldsymbol{\nabla}_\parallel\cdot\mathbf{F}(\mathbf{r})\,\mathrm{d}^2\mathbf{r} = \oint_{\partial S}\hat{\mathbf{n}}_{\partial S}\cdot\mathbf{F}(\mathbf{r})\,\mathrm{d}\mathbf{r}$, which applies to smooth vector functions $\mathbf{F}$ over 2D surfaces $S$ embedded in 3D, with associated line periphery $\partial S$ equipped with edge normal $\hat{\mathbf{n}}_{\partial S}$ ($\equiv \hat{\mathbf{t}}\times\hat{\mathbf{n}}$, i.e. expressible via the edge tangent $\hat{\mathbf{t}}$ to $\partial S$ and the surface normal $\hat{\mathbf{n}}$ to $S$). Presently, we have $S = \partial\Omega$ and $\partial S = \emptyset$.

[8] In principle, solutions with $\Lambda^{(0)} = \pm 2\pi$ may exist, though they are trivial in the sense that they correspond to diverging or vanishing dielectric properties, allowable only if $\varepsilon_\mathrm{d}/\varepsilon_\mathrm{m}\to\infty$ or $\varepsilon_\mathrm{m}/\varepsilon_\mathrm{d}\to\infty$.

## V. REPRESENTATIONS OF THE COULOMB INTERACTION IN SYMMETRIC GEOMETRIES

In deriving the analytical results presented in Table I of the main text, the following useful representations of the Coulomb interaction $g(\mathbf{r},\mathbf{r}')$ were employed [S8]:

$$g(\mathbf{r},\mathbf{r}') \equiv \frac{1}{|\mathbf{r}-\mathbf{r}'|} = \frac{1}{2\pi}\int_{\mathbb{R}^2} \frac{1}{k_\parallel} \mathrm{e}^{-k_\parallel|z-z'|}\mathrm{e}^{\mathrm{i}\mathbf{k}_\parallel\cdot(\mathbf{r}_\parallel-\mathbf{r}'_\parallel)}\mathrm{d}^2\mathbf{k}_\parallel, \tag{S31a}$$

$$= \frac{1}{\pi}\sum_{m=-\infty}^{\infty} \mathrm{e}^{\mathrm{i}m(\varphi-\varphi')}\int_{-\infty}^{\infty} \mathrm{e}^{\mathrm{i}k_z(z-z')} I_m(k_z r_{\parallel<})K_m(k_z r_{\parallel>})\,\mathrm{d}k_z, \tag{S31b}$$

$$= 4\pi\sum_{l=0}^{\infty}\sum_{m=-l}^{l}\frac{1}{2l+1}\overline{Y_l^m(\theta',\varphi')}Y_l^m(\theta,\varphi)\frac{r_<^l}{r_>^{l+1}}, \tag{S31c}$$

with utility to systems of planar, cylindrical, and spherical symmetry, respectively. Here, in-plane coordinates are indicated by $\parallel$-subscripts, azimuthal angles by $\varphi$, polar angles by $\theta$, lesser/greater lengths by $r_< \equiv \min(|\mathbf{r}|,|\mathbf{r}'|)$ and $r_> \equiv \max(|\mathbf{r}|,|\mathbf{r}'|)$, modified Bessel functions by $K_m$ and $I_m$, and spherical harmonics by $Y_l^m$.

## VI. COMPUTING FEIBELMAN *d*-PARAMETERS

To compute the Feibelman $d$-parameters of the materials discussed in Fig. 3 of the main text we employ time-dependent density functional theory (TDDFT). The calculations incorporate three central approximations: (1) the jellium approximation of the positive ionic background, (2) the semiclassical polarizable medium approximation (SPMA) of the valence electrons, and (3) the adiabatic local density approximation (ALDA)[9] of the exchange-correlation (xc) functional. The planar-interface implementation of TDDFT consistent with these approximations is well-described in several references [S11; S12]. For completeness, we nevertheless provide a brief summary of the central aspects, focusing in particular on the SPMA. Our intention is not to detail a practical numerical routine, the former references achieve this admirably, but rather to describe the physical content clearly and concisely.

For the semi-infinite planar metal-dielectric system, the positive ionic background is a function solely of $x$, the coordinate normal to the interface at $x = 0$. In the jellium approximation, the positive ionic background is assumed uniform, with value $n_{\mathrm{ion}}$ in the metallic region:

$$n_+(x) = \begin{cases} n_{\mathrm{ion}} & x<0 \quad \text{(metal region)},\\ 0 & x>0 \quad \text{(dielectric region)}, \end{cases} \tag{S32}$$

We note that $n_{\mathrm{ion}}$ acts to neutralize only the conduction electrons, leaving lower-lying orbitals (valence electrons) unaccounted. Instead, in the SPMA the polarization contribution of the valence electrons is included semiclassically through a “bound charge” dielectric contribution $\varepsilon_{\mathrm{m}}^{\mathrm{b}}$, acting in the region $x < x_{\mathrm{b}}$. For simple metals such as Na and Al, the polarization of the valence electrons can be neglected, and accordingly $\varepsilon_{\mathrm{m}}^{\mathrm{b}} = 1$. For Ag, the contribution from the 4d-band valence electrons is significant and non-negligible. The value of $\varepsilon_{\mathrm{m}}^{\mathrm{b}}$ can be inferred approximately by comparison with the experimentally measured dielectric function. Concretely, $\varepsilon_{\mathrm{m}}^{\mathrm{b}}$ accounts for all non-Drude features in the measured dielectric function $\varepsilon_{\mathrm{m}}$ in the sense:

$$\varepsilon_{\mathrm{m}}(\omega) \equiv \varepsilon_{\mathrm{m}}^{\mathrm{b}}(\omega) - \frac{\omega_{\mathrm{p}}^2}{\omega(\omega+\mathrm{i}\gamma)},$$

where, for Ag, $\hbar\omega_{\mathrm{p}} = \hbar\sqrt{e^2 n_{\mathrm{ion}}/\varepsilon_0 m_{\mathrm{e}}} \approx 9.02\,\mathrm{eV}$ (*un*screened plasma frequency) and $\hbar\gamma = 22\,\mathrm{meV}$ (Drude decay rate); in addition, we impose the constraint that $\mathrm{Im}\,\varepsilon_{\mathrm{m}}^{\mathrm{b}} = 0$ for energies below the onset (at

[9] TDDFT operated at the ALDA level is conventionally contracted as ‘time-dependent local density approximation’ (TDLDA).

3.7 eV) of interband transitions from 4d bands (to eliminate a small $\gamma$-dependent offset from zero). The frequency-dependence of $\varepsilon_{\rm m}^{\rm b}$ consistent with these choices – and the measurements of Johnson and Christy [S13] – is illustrated in Fig. S2a. Nondispersive behavior is assumed for energies below $\hbar\omega_{\rm static} \approx 2.5$ eV, such that $\varepsilon_{\rm m}^{\rm b}(\omega < \omega_{\rm static}) \approx 3.66$.

The spatial restriction of this bound contribution to $x < x_{\rm b}$ rather than to $x < 0$ is motivated by the stronger spatial localization of the valence bands relative to the conduction bands. Following Liebsch [S11], it is chosen as $x_{\rm b} = -1.18$ Å, corresponding to the half-distance between neighboring Ag(111) crystal planes. The dielectric contribution *not* due to conduction electrons, i.e. the bound or background dielectric contribution, then finally assumes the following $x$-dependence:

$$\varepsilon_{\rm s}(x,\omega) = \begin{cases} \varepsilon_{\rm m}^{\rm b}(\omega) & x < x_{\rm b}, \\ 1 & x_{\rm b} < x < 0, \\ \varepsilon_{\rm d} & x > 0, \end{cases} \tag{S33}$$

where $\varepsilon_{\rm d}$ is the dielectric function of the adjacent dielectric region. In the following, $\varepsilon_{\rm s}(x,\omega)$ enters the (TD)DFT calculations as a semiclassical *s*creening mechanism for the conduction electrons.

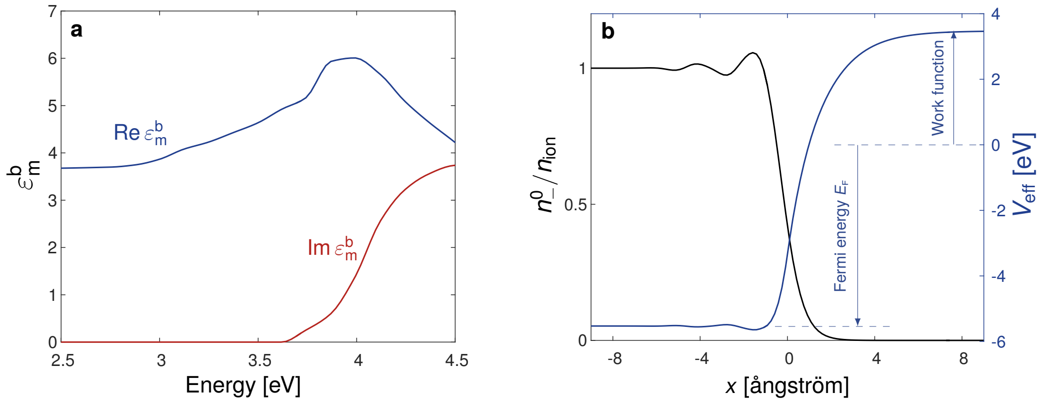


FIG. S2 **a**, Frequency-dependent bound dielectric contribution $\varepsilon_{\rm m}^{\rm b}$ of Ag due to 4d valence electrons. **b**, Calculated ground-state conduction electron density $n_-^0$ and effective potential $V_{\rm eff}$ of the semi-infinite Ag ($x < 0$)/vacuum ($x > 0$) setup. The 4d valence electrons are accounted for within the SPMA via $\varepsilon_{\rm s}(x,\omega = 0)$, through screening of the conduction electrons in the region $x < x_{\rm b}$ ($= -1.18$ Å). The work function indicated in the $V_{\rm eff}$ profile is 3.47 eV.

In the absence of external perturbations, the conduction electrons are described by a set of Kohn–Sham orbitals $\psi_\kappa(x)e^{i(k_y y + k_z z)}$ governed by [S14]

$$\left\{-\frac{\hbar^2}{2m_{\rm e}}\frac{{\rm d}^2}{{\rm d}^2x} - e\phi(x) + V_{\rm xc}\big[n_-^0(x)\big]\right\}\psi_\kappa(x) = \epsilon_\kappa\psi_\kappa(x), \tag{S34}$$

with eigenvalue $\epsilon_\kappa \equiv \hbar^2\kappa^2/2m_{\rm e}$ and orbital kinetic energy $E_{\kappa,k_y,k_z} \equiv \hbar^2(\kappa^2 + k_y^2 + k_z^2)/2m_{\rm e}$. Here $n_-^0$ is the ground-state density of the conduction electrons – given by the summation over occupied states below the Fermi level $\mu_{\rm F}$ ($\equiv -e\phi(-\infty) + V_{\rm xc}[n_{\rm ion}] + E_{\rm F}$, with Fermi energy $E_{\rm F}$) – reducing, at zero temperature, to

$$n_-^0(x) = \frac{1}{\pi^2}\int_0^{k_{\rm F}} (k_{\rm F}^2 - \kappa^2)|\psi_i(x)|^2\,{\rm d}\kappa, \tag{S35}$$

where $\hbar^2 k_{\rm F}^2/2m_{\rm e} \equiv E_{\rm F}$ defines the Fermi momentum. The self-consistent potential $\phi(x)$ satisfies a screened Poisson equation:

$$\frac{\rm d}{{\rm d}x}\left[\varepsilon_{\rm s}(x,\omega = 0)\frac{\rm d}{{\rm d}x}\phi(x)\right] = -e\left[n_-^0(x) - n_+(x)\right]. \tag{S36}$$

Finally, $V_{\rm xc}$ is chosen as the (LDA) Gunnarsson–Lundqvist xc-functional [S15]. In Fig. S2b, we show the computed ground state density of conduction electrons in the semi-infinite Ag-vacuum scenario, along its

corresponding effective potential $V_{\text{eff}}(x) \equiv -e\phi(x) + V_{\text{xc}}[n_-^0(x)] - \mu_{\text{F}}$. The work function of Ag obtained from this calculation is 3.47 eV; roughly 1 eV below the experimentally established value. The discrepancy is due to the coarse surface treatment inherent to the jellium-SPMA-LDA combination. Nevertheless, the influence of this discrepancy on plasmon dynamics is minor, as established by the agreement obtained between this scheme and numerous experimental studies of planar Ag surfaces[10] [S11; S17; S18].

To consider response dynamics, we next introduce a time-varying perturbation due to an external electric potential $\phi^{\text{ext}}(x,\omega)\text{e}^{-\text{i}\omega t}$. We consider $\phi^{\text{ext}}$ as invariant along the $y$ and $z$ coordinates, since our aim is to obtain the $d$-parameters in the limit $k \to 0$. In that case, $\phi^{\text{ext}}$ is given by

$$\phi^{\text{ext}}(x,\omega) = x \begin{cases} \frac{2}{\varepsilon_{\text{d}}-\varepsilon_{\text{m}}^{\text{b}}(\omega)} & x < x_{\text{b}}, \\ \frac{2\varepsilon_{\text{d}}\varepsilon_{\text{m}}^{\text{b}}(\omega)}{\varepsilon_{\text{d}}-\varepsilon_{\text{m}}^{\text{b}}(\omega)} & x_{\text{b}} < x < 0, \\ 1 - \frac{\varepsilon_{\text{d}}-\varepsilon_{\text{m}}^{\text{b}}(\omega)}{\varepsilon_{\text{d}}-\varepsilon_{\text{m}}^{\text{b}}(\omega)} & x > 0, \end{cases} \tag{S37}$$

which represents the potential generated by a charge sheet at $x \to \infty$ in the dielectric environment $\varepsilon_{\text{s}}(x,\omega)$. In response to $\phi^{\text{ext}}$ the conduction electron density $n_-(x,t) = n_-^0(x) + \delta n_-(x,t)$ develops an induced, time-varying component $\delta n_-(x,t) = \delta n_-(x,\omega)\text{e}^{-\text{i}\omega t}$ equaling (within linear response theory)

$$\delta n_-(x,\omega) = -e \int \chi(x,x';\omega)\phi^{\text{ext}}(x,\omega)\,\text{d}x', \tag{S38}$$

expressed through the interacting density-density response function $\chi$, obeying

$$\chi(x,x';\omega) = \chi^0(x,x';\omega) + \iint \chi^0(x,x_1;\omega)\big[-e^2 g(x_1,x_2;\omega) + f_{\text{xc}}[n_-](x_1,x_2;\omega)\big]\chi(x_2,x';\omega)\,\text{d}x_1\text{d}x_2\,,$$

with xc-kernel $f_{\text{xc}}[n_-](x_1,x_2;t-t') \equiv \frac{\delta V_{\text{xc}}[n_-](x_1,t)}{\delta n_-(x_2,t')}$; within ALDA, its frequency-representation simplifies to $f_{\text{xc}}[n_-](x_1,x_2;\omega) = \frac{\delta V_{\text{xc}}[n_-(x_1,\omega)]}{\delta n_-(x_2,\omega)}\delta(x_1-x_2)$. Lastly, $g(x,x';\omega)$ is the Green function of the 1D screened Poisson equation:

$$\frac{\text{d}}{\text{d}x}\left[\varepsilon_{\text{s}}(x,\omega)\frac{\text{d}}{\text{d}x}g(x,x';\omega)\right] = \delta(x-x'). \tag{S39}$$

The noninteracting response function $\chi^0$ can be constructed directly from the Kohn–Sham orbitals [S19].

To obtain the *total* induced density, summing induced densities of both conduction and valence electrons, we observe that once the induced conduction density $\delta n_-$ is computed, the induced electric potential $\phi^{\text{ind}}$ follows straightforwardly from the screened Poisson equation:

$$\frac{\text{d}}{\text{d}x}\left[\varepsilon_{\text{s}}(x,\omega)\frac{\text{d}}{\text{d}x}\phi^{\text{ind}}(x,\omega)\right] = e\delta n_-(x), \tag{S40}$$

from which the total induced (charge) density $\rho = -e(\delta n_- + \text{induced valence density})$ follow via

$$\rho(x,\omega) = -\varepsilon_0\frac{\text{d}^2}{\text{d}x^2}\phi^{\text{ind}}(x,\omega). \tag{S41}$$

Equipped with $\rho(x,\omega)$, $d_\perp$ can then in principle be calculated directly from its definition, Eq. (1). We note, however, that direct evaluation of $d_\perp$ is not favorable due to Friedel oscillations of the induced charge which decay only slowly inside the metal. Liebsch proposed an elegant scheme to avoid this numerical difficulty by utilizing the dynamic force sum rule [S12] which we have followed in our numerical implementation.

---

[10] Nevertheless, we hasten to add that non-jellium calculations of the $d$-parameters, with explicit incorporation of lower-lying orbitals, would represent a highly interesting and pertinent extension of the state-of-the-art. Such calculations should be feasible with existing numerical TDDFT packages [S16], e.g. through consideration of thick slabs. Furthermore, explicit account of the atomic structure poses additional interesting questions, such as the crystal-face dependence of the $d$-parameters. Evidently, several semiclassical approximations conspire in the jellium-SPMA combination, which would be preferable to avoid from an ab initio perspective: the establishment of an ab initio inventory of $d$-parameters in various metals appears a worthwhile goal in our view.

Finally, due to the approximations inherent in the SPMA, the parallel $d$-parameter, $d_\parallel$, which ordinarily vanishes at charge-neutral interfaces, acquires a finite, nonzero value which must be included for consistency. In the limit of $k \to 0$, it has a simple entirely classical expression [S12]:

$$d_\parallel(\omega) = x_\mathrm{b}\frac{\varepsilon_\mathrm{m}^\mathrm{b}(\omega) - 1}{\varepsilon_\mathrm{m}(\omega) - \varepsilon_\mathrm{d}}, \tag{S42}$$

with the minor subtlety that the evaluation of $\varepsilon_\mathrm{m}^{(\mathrm{b})}$ assumes a vanishing Drude decay rate; a choice necessitated by consistency due to its exclusion from the TDDFT evaluation of $d_\perp$.

## VII. COMPARISON WITH TDDFT CALCULATIONS IN NA NANOSPHERES

Figure S3 extends the comparison between the presently introduced $d$-parameter method and full TDLDA calculations (with geometry-specific orbitals), here exemplified by the results of Weick *et al.* [S20], to smaller nanosphere radii than those considered in the main text. The agreement is excellent; this highlights the exceptional quality of the present analytical approach relative to well-established computationally intensive methods such as jellium TDDFT with geometry-specific orbitals. The negligible difference between $d$-parameter method calculations at $r_s = 3.93$ and $r_s = 4$ justifies the comparison in Fig. 3 of the main text between Weick's $r_s = 3.93$ data and the $r_s = 4$ case considered there.

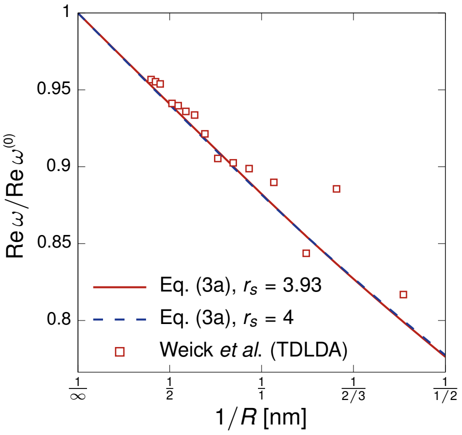


FIG. S3 Spectral evolution of the dipole plasmon resonance in Na ($r_s = 3.93$) nanospheres with inverse nanosphere radius $1/R$. Results of the present $d$-parameter method, obtained by solving Eq. (3a) of the main text numerically, are compared with the TDLDA jellium calculations reported previously by Weick *et al.* [S20]. A calculation for $r_s = 4$ is also included, showing negligible difference from the $r_s = 3.93$ case.

### References


[S1] P.J. Feibelman, *Surface electromagnetic fields,* Prog. Surf. Sci. **12**, 287 (1982).
[S2] A. Liebsch, *Electronic Excitations at Metal Surfaces*, Physics of Solids and Liquids (Springer, 1997).
[S3] P. Apell, *A simple derivation of the surface contribution to the reflectivity of a metal, and its use in the van der Waals interaction,* Physica Scripta **24**, 795 (1981).
[S4] K. Kempa and W.L. Schaich, *Calculation of corrections to Fresnel optics from density response,* Phys. Rev. B **34**, 547 (1986).
[S5] I.S. Gradshteyn and I.M. Ryzhik, *Table of Integrals, Series, and Products*, 7th ed. (Academic Press, 2007).
[S6] W. Yan, M. Wubs, and N.A. Mortensen, *Projected dipole model for quantum plasmonics,* Phys. Rev. Lett. **115**, 137403 (2015).
[S7] F.H.L. Koppens, D.E. Chang, and F.J. García de Abajo, *Graphene plasmonics: a platform for strong light–matter interactions,* Nano Lett. **11**, 3370 (2011).
[S8] J.D. Jackson, *Classical Electrodynamics*, 3rd ed. (John Wiley & Sons, 1999).
[S9] F. Ouyang and M. Isaacson, *Surface plasmon excitation of objects with arbitrary shape and dielectric constant,* Philos. Mag. B **60**, 481 (1989).

[S10] O.D. Kellogg, *Foundations of Potential Theory* (Springer, 1967).
[S11] A. Liebsch, *Surface-plasmon dispersion and size dependence of Mie resonance: silver versus simple metals,* Phys. Rev. B **48**, 11317 (1993).
[S12] A. Liebsch and W.L. Schaich, *Influence of a polarizable medium on the nonlocal optical response of a metal surface,* Phys. Rev. B **52**, 14219 (1995).
[S13] P.B. Johnson and R.W. Christy, *Optical constants of the noble metals,* Phys. Rev. B **6**, 4370 (1972).
[S14] N.D. Lang and W. Kohn, *Theory of metal surfaces: charge density and surface energy,* Phys. Rev. B **1**, 4555 (1970).
[S15] O. Gunnarsson and B.I. Lundqvist, *Exchange and correlation in atoms, molecules, and solids by the spin-density-functional formalism,* Phys. Rev. B **13**, 4274 (1976).
[S16] J. Yan, K.W. Jacobsen, and K.S. Thygesen, *First-principles study of surface plasmons on Ag(111) and H/Ag(111),* Phys. Rev. B **84**, 235430 (2011).
[S17] K.-D. Tsuei, E.W. Plummer, A. Liebsch, E. Pehlke, K. Kempa, and P. Bakshi, *The normal modes at the surface of simple metals,* Surf. Sci. **247**, 302 (1991).
[S18] D. Jin, Q. Hu, D. Neuhauser, F. von Cube, Y. Yang, R. Sachan, T.S. Luk, D.C. Bell, and N.X. Fang, *Quantum-spillover-enhanced surface-plasmonic absorption at the interface of silver and high-index dielectrics,* Phys. Rev. Lett. **115**, 193901 (2015).
[S19] A. Liebsch, *Dynamical screening at simple-metal surfaces,* Phys. Rev. B **36**, 7378 (1987).
[S20] G. Weick, G.-L. Ingold, R.A. Jalabert, and D. Weinmann, *Surface plasmon in metallic nanoparticles: Renormalization effects due to electron-hole excitations,* Phys. Rev. B **74**, 165421 (2006).
